# Supplementary material for: Theory of magnetic properties in QED environments: application to molecular aromaticity
Source: arXiv:2402.10599 source file (2024-02-16)
Supplement: Supplementary file 1 [file SI.pdf]

# Supporting information for Theory of magnetic properties in QED environments: application to molecular aromaticity

Alberto Barlini,† Andrea Bianchi,† Enrico Ronca,*,‡ and Henrik Koch*,¶

†*Scuola Normale Superiore, Pisa, Italy*

‡*Dipartimento di Chimica, Biologia e Biotecnologie, Università degli Studi di Perugia, Perugia, Italy*

¶*Department of Chemistry, Norwegian University of Science and Technology, Trondheim, Norway*

E-mail: enrico.ronca@unipg.it; henrik.koch@ntnu.no

## On the cavity field approximation

Consider the following expressions for the electric and magnetic field

$$\mathbf{E}\left(\mathbf{r}_i\right) = i\sum_{\mathbf{k}\lambda}\omega_{\mathbf{k}}\mathcal{A}_{\mathbf{k}}\boldsymbol{\epsilon}_\lambda\left(b_{\mathbf{k}\lambda} - b^\dagger_{\mathbf{k}\lambda}\right) + \frac{1}{2}\sum_{\mathbf{k}\lambda}\omega_{\mathbf{k}}\mathcal{A}_{\mathbf{k}}\left(\mathbf{r}_i \times \left(\mathbf{k}\times\boldsymbol{\epsilon}_\lambda\right)\right)\left(b_{\mathbf{k}\lambda} + b^\dagger_{\mathbf{k}\lambda}\right) \tag{1}$$

$$\mathbf{B}\left(\mathbf{r}_i\right) = i\sum_{\mathbf{k}\lambda}\mathcal{A}_{\mathbf{k}}\left(\mathbf{k}\times\boldsymbol{\epsilon}_\lambda\right)\left(b_{\mathbf{k}\lambda} - b^\dagger_{\mathbf{k}\lambda}\right). \tag{2}$$

By substituting Eq. 1 and Eq. 2 in the Maxwell's equations expressed in atomic units, we obtain

$$\nabla\cdot\mathbf{E} = 0 \tag{3}$$

$$\nabla\cdot\mathbf{B} = 0 \tag{4}$$

$$\nabla\times\mathbf{E} = -\frac{\partial\mathbf{B}}{\partial t} \tag{5}$$

$$\nabla\times\mathbf{B} \neq -\frac{1}{c^2}\frac{\partial\mathbf{E}}{\partial t}. \tag{6}$$

Here, Eq. 6 is not fulfilled. Indeed, the left-hand side and the right-hand side read as

$$\nabla \times \mathbf{B} = 0 \tag{7}$$

$$-\frac{1}{c^2}\frac{\partial \mathbf{E}}{\partial t} = \frac{1}{c^2}\sum_{\mathbf{k}\lambda}\omega_{\mathbf{k}}^2 \mathcal{A}_{\mathbf{k}} \boldsymbol{\epsilon}_\lambda \left(b_{\mathbf{k}\lambda} - b_{\mathbf{k}\lambda}^\dagger\right) + \frac{i}{2}\sum_{\mathbf{k}\lambda}\omega_{\mathbf{k}}^2 \mathcal{A}_{\mathbf{k}} \left(\mathbf{r}_i \times (\mathbf{k} \times \boldsymbol{\epsilon}_\lambda)\right)\left(b_{\mathbf{k}\lambda} - b_{\mathbf{k}\lambda}^\dagger\right), \tag{8}$$

where the time dependence of the electric field in Eq. 1 resides in the photon operators

$$b = \tilde{b}\,\exp\left(i\omega t\right) \tag{9}$$

$$b^\dagger = \tilde{b}^\dagger\,\exp\left(-i\omega t\right). \tag{10}$$

## B3LYP/def2-SVP optimized geometries

This section reports the optimized geometries in angstrom of the examined hydrocarbons used in the HF and QED-HF magnetizability.

**Methane**

| | | | |
|---|---|---|---|
| C | 0.000000 | -0.000000 | 0.000000 |
| H | -0.000000 | -0.897870 | -0.634876 |
| H | -0.000000 | 0.897870 | -0.634876 |
| H | -0.897870 | -0.000000 | 0.634876 |
| H | 0.897870 | 0.000000 | 0.634876 |

**Ethylene**

| | | | |
|---|---|---|---|
| C | -0.666616 | 0.000006 | -0.000000 |
| C | 0.666649 | -0.000007 | 0.000001 |
| H | -1.242769 | -0.928617 | 0.070771 |
| H | -1.242751 | 0.928640 | -0.070773 |
| H | 1.242801 | 0.928616 | -0.070771 |
| H | 1.242786 | -0.928638 | 0.070772 |

**Acethylene**

| | | | |
|---|---|---|---|
| C | -0.604660 | 0.000000 | -0.000005 |
| C | 0.604660 | 0.000000 | 0.000005 |
| H | -1.679229 | 0.000000 | -0.000099 |
| H | 1.679229 | 0.000000 | 0.000099 |

**Benzene**

| | | | |
|---|---|---|---|
| C | -1.216810 | -0.690500 | 0.000008 |
| C | -1.206456 | 0.708523 | 0.000022 |
| C | -0.010350 | -1.398981 | -0.000002 |
| C | 0.010407 | 1.399004 | 0.000016 |
| C | 1.206498 | -0.708489 | -0.000002 |
| C | 1.216858 | 0.690526 | 0.000009 |
| H | -2.167931 | -1.230304 | 0.000010 |
| H | -2.149461 | 1.262372 | 0.000031 |
| H | -0.018509 | -2.492589 | -0.000015 |
| H | 0.018492 | 2.492614 | 0.000026 |
| H | 2.149504 | -1.262340 | -0.000005 |
| H | 2.167958 | 1.230365 | 0.000003 |

## NEB-TS optimized geometries

This section reports the optimized geometries in angstrom of the trimerization reaction pathway. The first of the following geometries corresponds to the transition state geometry.

**Transition state geometry**

| | | | |
|---|---|---|---|
| C | 1.699255 | 0.616421 | 0.000000 |
| C | 1.699255 | -0.616421 | 0.000000 |
| C | -0.315404 | -1.780419 | -0.000000 |
| C | -0.315403 | 1.780419 | 0.000000 |
| C | -1.383900 | -1.165609 | 0.000000 |
| C | -1.383900 | 1.165609 | -0.000000 |
| H | 2.160072 | -1.586595 | 0.000000 |
| H | 2.160072 | 1.586595 | -0.000000 |
| H | 0.294821 | 2.664332 | 0.000000 |
| H | 0.294821 | -2.664333 | -0.000000 |
| H | -2.454316 | 1.077612 | -0.000000 |
| H | -2.454316 | -1.077612 | 0.000000 |

**Reaction patways geometries**

| | | | |
|---|---|---|---|
| C | 2.141858 | 0.592962 | 0.000000 |
| C | 2.141858 | -0.592962 | 0.000000 |
| C | -0.557895 | -2.154007 | -0.000000 |
| C | -0.557895 | 2.154007 | -0.000000 |
| C | -1.583800 | -1.561192 | -0.000000 |
| C | -1.583800 | 1.561192 | -0.000000 |
| H | 2.194181 | -1.645536 | 0.000000 |
| H | 2.194181 | 1.645536 | 0.000000 |
| H | 0.323820 | 2.723740 | 0.000000 |
| H | 0.323820 | -2.723740 | 0.000000 |
| H | -2.519930 | 1.080194 | -0.000000 |
| H | -2.519930 | -1.080194 | -0.000000 |

| | | | |
|---|---|---|---|
| C | 2.121582 | 0.593797 | 0.000000 |
| C | 2.121582 | -0.593797 | 0.000000 |
| C | -0.547026 | -2.136804 | -0.000000 |
| C | -0.547026 | 2.136804 | -0.000000 |
| C | -1.574396 | -1.543155 | -0.000000 |
| C | -1.574396 | 1.543155 | -0.000000 |
| H | 2.194029 | -1.644578 | 0.000000 |
| H | 2.194029 | 1.644578 | 0.000000 |
| H | 0.323149 | 2.723100 | 0.000000 |
| H | 0.323149 | -2.723100 | 0.000000 |
| H | -2.519066 | 1.080463 | -0.000000 |
| H | -2.519066 | -1.080463 | -0.000000 |

| | | | |
|---|---|---|---|
| C | 2.101311 | 0.594709 | 0.000000 |
| C | 2.101311 | -0.594709 | 0.000000 |
| C | -0.536093 | -2.119645 | -0.000000 |
| C | -0.536093 | 2.119645 | -0.000000 |
| C | -1.565062 | -1.525085 | -0.000000 |
| C | -1.565062 | 1.525085 | -0.000000 |
| H | 2.194095 | -1.643372 | 0.000000 |
| H | 2.194095 | 1.643372 | 0.000000 |
| H | 0.322149 | 2.722526 | 0.000000 |
| H | 0.322149 | -2.722526 | 0.000000 |
| H | -2.518098 | 1.081048 | -0.000000 |
| H | -2.518098 | -1.081048 | -0.000000 |

| | | | |
|---|---|---|---|
| C | 2.081044 | 0.595693 | 0.000000 |
| C | 2.081044 | -0.595693 | 0.000000 |
| C | -0.525099 | -2.102525 | -0.000000 |
| C | -0.525099 | 2.102525 | -0.000000 |
| C | -1.555791 | -1.506983 | -0.000000 |
| C | -1.555791 | 1.506983 | -0.000000 |
| H | 2.194357 | -1.641897 | 0.000000 |
| H | 2.194357 | 1.641897 | 0.000000 |
| H | 0.320815 | 2.721987 | 0.000000 |
| H | 0.320815 | -2.721987 | 0.000000 |
| H | -2.516994 | 1.081940 | -0.000000 |
| H | -2.516994 | -1.081940 | -0.000000 |

| | | | |
|---|---|---|---|
| C | 2.060777 | 0.596747 | 0.000000 |
| C | 2.060777 | -0.596747 | 0.000000 |
| C | -0.514046 | -2.085442 | -0.000000 |
| C | -0.514046 | 2.085442 | -0.000000 |
| C | -1.546581 | -1.488848 | -0.000000 |
| C | -1.546581 | 1.488848 | -0.000000 |
| H | 2.194792 | -1.640136 | 0.000000 |
| H | 2.194792 | 1.640136 | 0.000000 |
| H | 0.319143 | 2.721455 | 0.000000 |
| H | 0.319143 | -2.721455 | 0.000000 |
| H | -2.515728 | 1.083128 | -0.000000 |
| H | -2.515728 | -1.083128 | -0.000000 |

| | | | |
|---|---|---|---|
| C | 2.040510 | 0.597868 | 0.000000 |
| C | 2.040510 | -0.597868 | 0.000000 |
| C | -0.502935 | -2.068392 | -0.000000 |
| C | -0.502935 | 2.068392 | -0.000000 |
| C | -1.537428 | -1.470679 | -0.000000 |
| C | -1.537428 | 1.470679 | -0.000000 |
| H | 2.195379 | -1.638071 | 0.000000 |
| H | 2.195379 | 1.638071 | 0.000000 |
| H | 0.317128 | 2.720903 | 0.000000 |
| H | 0.317128 | -2.720903 | 0.000000 |
| H | -2.514274 | 1.084601 | -0.000000 |
| H | -2.514274 | -1.084601 | -0.000000 |

| | | | |
|---|---|---|---|
| C | 2.020240 | 0.599052 | 0.000000 |
| C | 2.020240 | -0.599052 | 0.000000 |
| C | -0.491767 | -2.051372 | -0.000000 |
| C | -0.491767 | 2.051372 | -0.000000 |
| C | -1.528328 | -1.452477 | -0.000000 |
| C | -1.528328 | 1.452477 | -0.000000 |
| H | 2.196097 | -1.635685 | 0.000000 |
| H | 2.196097 | 1.635685 | 0.000000 |
| H | 0.314768 | 2.720303 | 0.000000 |
| H | 0.314768 | -2.720303 | 0.000000 |
| H | -2.512606 | 1.086351 | -0.000000 |
| H | -2.512606 | -1.086351 | -0.000000 |

| | | | |
|---|---|---|---|
| C | 1.999967 | 0.600298 | 0.000000 |
| C | 1.999967 | -0.600298 | 0.000000 |
| C | -0.480544 | -2.034380 | -0.000000 |
| C | -0.480544 | 2.034380 | -0.000000 |
| C | -1.519279 | -1.434241 | -0.000000 |
| C | -1.519279 | 1.434241 | -0.000000 |
| H | 2.196926 | -1.632964 | 0.000000 |
| H | 2.196926 | 1.632964 | 0.000000 |
| H | 0.312060 | 2.719630 | 0.000000 |
| H | 0.312060 | -2.719630 | 0.000000 |
| H | -2.510702 | 1.088365 | -0.000000 |
| H | -2.510702 | -1.088365 | -0.000000 |

| | | | |
|---|---|---|---|
| C | 1.979692 | 0.601603 | 0.000000 |
| C | 1.979692 | -0.601603 | 0.000000 |
| C | -0.469270 | -2.017417 | -0.000000 |
| C | -0.469270 | 2.017417 | -0.000000 |
| C | -1.510281 | -1.415974 | -0.000000 |
| C | -1.510281 | 1.415974 | -0.000000 |
| H | 2.197844 | -1.629894 | 0.000000 |
| H | 2.197844 | 1.629894 | 0.000000 |
| H | 0.309003 | 2.718861 | 0.000000 |
| H | 0.309003 | -2.718861 | 0.000000 |
| H | -2.508542 | 1.090634 | -0.000000 |
| H | -2.508542 | -1.090634 | -0.000000 |

| | | | |
|---|---|---|---|
| C | 1.959418 | 0.602965 | 0.000000 |
| C | 1.959418 | -0.602965 | 0.000000 |
| C | -0.457947 | -2.000485 | -0.000000 |
| C | -0.457947 | 2.000485 | -0.000000 |
| C | -1.501331 | -1.397680 | -0.000000 |
| C | -1.501331 | 1.397680 | -0.000000 |
| H | 2.198835 | -1.626463 | 0.000000 |
| H | 2.198835 | 1.626463 | 0.000000 |
| H | 0.305597 | 2.717972 | 0.000000 |
| H | 0.305597 | -2.717972 | 0.000000 |
| H | -2.506102 | 1.093145 | -0.000000 |
| H | -2.506102 | -1.093145 | -0.000000 |

| | | | |
|---|---|---|---|
| C | 1.939150 | 0.604382 | 0.000000 |
| C | 1.939150 | -0.604382 | 0.000000 |
| C | -0.446581 | -1.983584 | -0.000000 |
| C | -0.446581 | 1.983584 | -0.000000 |
| C | -1.492431 | -1.379363 | -0.000000 |
| C | -1.492431 | 1.379363 | -0.000000 |
| H | 2.199876 | -1.622662 | 0.000000 |
| H | 2.199876 | 1.622662 | 0.000000 |
| H | 0.301842 | 2.716941 | 0.000000 |
| H | 0.301842 | -2.716941 | 0.000000 |
| H | -2.503367 | 1.095888 | -0.000000 |
| H | -2.503367 | -1.095888 | -0.000000 |

| | | | |
|---|---|---|---|
| C | 1.918893 | 0.605851 | 0.000000 |
| C | 1.918893 | -0.605851 | 0.000000 |
| C | -0.435175 | -1.966721 | -0.000000 |
| C | -0.435175 | 1.966721 | -0.000000 |
| C | -1.483582 | -1.361030 | -0.000000 |
| C | -1.483582 | 1.361030 | -0.000000 |
| H | 2.200951 | -1.618481 | 0.000000 |
| H | 2.200951 | 1.618481 | 0.000000 |
| H | 0.297742 | 2.715748 | 0.000000 |
| H | 0.297742 | -2.715748 | 0.000000 |
| H | -2.500318 | 1.098850 | -0.000000 |
| H | -2.500318 | -1.098850 | -0.000000 |

| | | | |
|---|---|---|---|
| C | 1.898654 | 0.607370 | 0.000000 |
| C | 1.898654 | -0.607370 | 0.000000 |
| C | -0.423735 | -1.949900 | -0.000000 |
| C | -0.423735 | 1.949900 | -0.000000 |
| C | -1.474786 | -1.342688 | -0.000000 |
| C | -1.474786 | 1.342688 | -0.000000 |
| H | 2.202041 | -1.613913 | 0.000000 |
| H | 2.202041 | 1.613913 | 0.000000 |
| H | 0.293298 | 2.714373 | 0.000000 |
| H | 0.293298 | -2.714373 | 0.000000 |
| H | -2.496942 | 1.102019 | -0.000000 |
| H | -2.496942 | -1.102019 | -0.000000 |

| | | | |
|---|---|---|---|
| C | 1.878443 | 0.608937 | 0.000000 |
| C | 1.878443 | -0.608937 | 0.000000 |
| C | -0.412268 | -1.933126 | -0.000000 |
| C | -0.412268 | 1.933126 | -0.000000 |
| C | -1.466044 | -1.324346 | -0.000000 |
| C | -1.466044 | 1.324346 | -0.000000 |
| H | 2.203129 | -1.608953 | 0.000000 |
| H | 2.203129 | 1.608953 | 0.000000 |
| H | 0.288517 | 2.712799 | 0.000000 |
| H | 0.288517 | -2.712799 | 0.000000 |
| H | -2.493223 | 1.105382 | -0.000000 |
| H | -2.493223 | -1.105382 | -0.000000 |

| | | | |
|---|---|---|---|
| C | 1.858269 | 0.610550 | 0.000000 |
| C | 1.858269 | -0.610550 | 0.000000 |
| C | -0.400779 | -1.916409 | -0.000000 |
| C | -0.400779 | 1.916409 | -0.000000 |
| C | -1.457360 | -1.306012 | -0.000000 |
| C | -1.457360 | 1.306012 | -0.000000 |
| H | 2.204197 | -1.603598 | 0.000000 |
| H | 2.204197 | 1.603598 | 0.000000 |
| H | 0.283403 | 2.711010 | 0.000000 |
| H | 0.283403 | -2.711010 | 0.000000 |
| H | -2.489151 | 1.108926 | -0.000000 |
| H | -2.489151 | -1.108926 | -0.000000 |

| | | | |
|---|---|---|---|
| C | 1.838142 | 0.612207 | 0.000000 |
| C | 1.838142 | -0.612207 | 0.000000 |
| C | -0.389276 | -1.899754 | -0.000000 |
| C | -0.389276 | 1.899754 | -0.000000 |
| C | -1.448737 | -1.287696 | -0.000000 |
| C | -1.448737 | 1.287696 | -0.000000 |
| H | 2.205229 | -1.597846 | 0.000000 |
| H | 2.205229 | 1.597846 | 0.000000 |
| H | 0.277965 | 2.708989 | 0.000000 |
| H | 0.277965 | -2.708989 | 0.000000 |
| H | -2.484716 | 1.112636 | -0.000000 |
| H | -2.484716 | -1.112636 | -0.000000 |

| | | | |
|---|---|---|---|
| C | 1.818072 | 0.613906 | 0.000000 |
| C | 1.818072 | -0.613906 | 0.000000 |
| C | -0.377767 | -1.883171 | -0.000000 |
| C | -0.377767 | 1.883171 | -0.000000 |
| C | -1.440180 | -1.269410 | -0.000000 |
| C | -1.440180 | 1.269410 | -0.000000 |
| H | 2.206208 | -1.591699 | 0.000000 |
| H | 2.206208 | 1.591699 | 0.000000 |
| H | 0.272211 | 2.706724 | 0.000000 |
| H | 0.272211 | -2.706724 | 0.000000 |
| H | -2.479912 | 1.116499 | -0.000000 |
| H | -2.479912 | -1.116499 | -0.000000 |

| | | | |
|---|---|---|---|
| C | 1.798073 | 0.615644 | 0.000000 |
| C | 1.798073 | -0.615644 | 0.000000 |
| C | -0.366259 | -1.866669 | -0.000000 |
| C | -0.366259 | 1.866669 | -0.000000 |
| C | -1.431691 | -1.251164 | -0.000000 |
| C | -1.431691 | 1.251164 | -0.000000 |
| H | 2.207119 | -1.585158 | 0.000000 |
| H | 2.207119 | 1.585158 | 0.000000 |
| H | 0.266152 | 2.704202 | 0.000000 |
| H | 0.266152 | -2.704202 | 0.000000 |
| H | -2.474732 | 1.120499 | -0.000000 |
| H | -2.474732 | -1.120499 | -0.000000 |

| | | | |
|---|---|---|---|
| C | 1.778157 | 0.617420 | 0.000000 |
| C | 1.778157 | -0.617420 | 0.000000 |
| C | -0.354760 | -1.850257 | -0.000000 |
| C | -0.354760 | 1.850257 | -0.000000 |
| C | -1.423276 | -1.232970 | -0.000000 |
| C | -1.423276 | 1.232970 | -0.000000 |
| H | 2.207948 | -1.578229 | 0.000000 |
| H | 2.207948 | 1.578229 | 0.000000 |
| H | 0.259800 | 2.701413 | 0.000000 |
| H | 0.259800 | -2.701413 | 0.000000 |
| H | -2.469172 | 1.124621 | -0.000000 |
| H | -2.469172 | -1.124621 | -0.000000 |

| | | | |
|---|---|---|---|
| C | 1.758336 | 0.619232 | 0.000000 |
| C | 1.758336 | -0.619232 | 0.000000 |
| C | -0.343279 | -1.833947 | -0.000000 |
| C | -0.343279 | 1.833947 | -0.000000 |
| C | -1.414940 | -1.214842 | -0.000000 |
| C | -1.414940 | 1.214842 | -0.000000 |
| H | 2.208678 | -1.570920 | 0.000000 |
| H | 2.208678 | 1.570920 | 0.000000 |
| H | 0.253169 | 2.698348 | 0.000000 |
| H | 0.253169 | -2.698348 | 0.000000 |
| H | -2.463235 | 1.128847 | -0.000000 |
| H | -2.463235 | -1.128847 | -0.000000 |

| | | | |
|---|---|---|---|
| C | 1.738630 | 0.621077 | 0.000000 |
| C | 1.738630 | -0.621077 | 0.000000 |
| C | -0.331827 | -1.817753 | -0.000000 |
| C | -0.331827 | 1.817753 | -0.000000 |
| C | -1.406690 | -1.196795 | -0.000000 |
| C | -1.406690 | 1.196795 | -0.000000 |
| H | 2.209296 | -1.563242 | 0.000000 |
| H | 2.209296 | 1.563242 | 0.000000 |
| H | 0.246276 | 2.695001 | 0.000000 |
| H | 0.246276 | -2.695001 | 0.000000 |
| H | -2.456921 | 1.133161 | -0.000000 |
| H | -2.456921 | -1.133161 | -0.000000 |

| | | | |
|---|---|---|---|
| C | 1.719064 | 0.622953 | 0.000000 |
| C | 1.719064 | -0.622953 | 0.000000 |
| C | -0.320417 | -1.801695 | -0.000000 |
| C | -0.320417 | 1.801695 | -0.000000 |
| C | -1.398536 | -1.178854 | -0.000000 |
| C | -1.398536 | 1.178854 | -0.000000 |
| H | 2.209790 | -1.555213 | 0.000000 |
| H | 2.209790 | 1.555213 | 0.000000 |
| H | 0.239145 | 2.691369 | 0.000000 |
| H | 0.239145 | -2.691369 | 0.000000 |
| H | -2.450240 | 1.137541 | -0.000000 |
| H | -2.450240 | -1.137541 | -0.000000 |

| | | | |
|---|---|---|---|
| C | 1.699662 | 0.624859 | 0.000000 |
| C | 1.699662 | -0.624859 | 0.000000 |
| C | -0.309066 | -1.785795 | -0.000000 |
| C | -0.309066 | 1.785795 | -0.000000 |
| C | -1.390491 | -1.161040 | -0.000000 |
| C | -1.390491 | 1.161040 | -0.000000 |
| H | 2.210145 | -1.546856 | 0.000000 |
| H | 2.210145 | 1.546856 | 0.000000 |
| H | 0.231799 | 2.687454 | 0.000000 |
| H | 0.231799 | -2.687454 | 0.000000 |
| H | -2.443206 | 1.141964 | -0.000000 |
| H | -2.443206 | -1.141964 | -0.000000 |

| | | | |
|---|---|---|---|
| C | 1.680442 | 0.626795 | 0.000000 |
| C | 1.680442 | -0.626795 | 0.000000 |
| C | -0.297778 | -1.770067 | -0.000000 |
| C | -0.297778 | 1.770067 | -0.000000 |
| C | -1.382562 | -1.143368 | -0.000000 |
| C | -1.382562 | 1.143368 | -0.000000 |
| H | 2.210351 | -1.538194 | 0.000000 |
| H | 2.210351 | 1.538194 | 0.000000 |
| H | 0.224268 | 2.683256 | 0.000000 |
| H | 0.224268 | -2.683256 | 0.000000 |
| H | -2.435831 | 1.146410 | -0.000000 |
| H | -2.435831 | -1.146410 | -0.000000 |

| | | | |
|---|---|---|---|
| C | 1.661397 | 0.628759 | 0.000000 |
| C | 1.661397 | -0.628759 | 0.000000 |
| C | -0.286554 | -1.754504 | -0.000000 |
| C | -0.286554 | 1.754504 | -0.000000 |
| C | -1.374744 | -1.125833 | -0.000000 |
| C | -1.374744 | 1.125833 | -0.000000 |
| H | 2.210396 | -1.529237 | 0.000000 |
| H | 2.210396 | 1.529237 | 0.000000 |
| H | 0.216563 | 2.678772 | 0.000000 |
| H | 0.216563 | -2.678772 | 0.000000 |
| H | -2.428121 | 1.150864 | -0.000000 |
| H | -2.428121 | -1.150864 | -0.000000 |

| | | | |
|---|---|---|---|
| C | 1.642500 | 0.630751 | 0.000000 |
| C | 1.642500 | -0.630751 | 0.000000 |
| C | -0.275382 | -1.739084 | -0.000000 |
| C | -0.275382 | 1.739084 | -0.000000 |
| C | -1.367026 | -1.108413 | -0.000000 |
| C | -1.367026 | 1.108413 | -0.000000 |
| H | 2.210272 | -1.519982 | 0.000000 |
| H | 2.210272 | 1.519982 | 0.000000 |
| H | 0.208685 | 2.673994 | 0.000000 |
| H | 0.208685 | -2.673994 | 0.000000 |
| H | -2.420068 | 1.155320 | -0.000000 |
| H | -2.420068 | -1.155320 | -0.000000 |

| | | | |
|---|---|---|---|
| C | 1.623733 | 0.632768 | 0.000000 |
| C | 1.623733 | -0.632768 | 0.000000 |
| C | -0.264251 | -1.723787 | -0.000000 |
| C | -0.264251 | 1.723787 | -0.000000 |
| C | -1.359394 | -1.091092 | -0.000000 |
| C | -1.359394 | 1.091092 | -0.000000 |
| H | 2.209974 | -1.510423 | 0.000000 |
| H | 2.209974 | 1.510423 | 0.000000 |
| H | 0.200636 | 2.668911 | 0.000000 |
| H | 0.200636 | -2.668911 | 0.000000 |
| H | -2.411664 | 1.159775 | -0.000000 |
| H | -2.411664 | -1.159775 | -0.000000 |

| | | | |
|---|---|---|---|
| C | 1.605091 | 0.634810 | 0.000000 |
| C | 1.605091 | -0.634810 | 0.000000 |
| C | -0.253161 | -1.708610 | -0.000000 |
| C | -0.253161 | 1.708610 | -0.000000 |
| C | -1.351846 | -1.073866 | -0.000000 |
| C | -1.351846 | 1.073866 | -0.000000 |
| H | 2.209492 | -1.500572 | 0.000000 |
| H | 2.209492 | 1.500572 | 0.000000 |
| H | 0.192427 | 2.663523 | 0.000000 |
| H | 0.192427 | -2.663523 | 0.000000 |
| H | -2.402915 | 1.164216 | -0.000000 |
| H | -2.402915 | -1.164216 | -0.000000 |

| | | | |
|---|---|---|---|
| C | 1.586584 | 0.636878 | 0.000000 |
| C | 1.586584 | -0.636878 | 0.000000 |
| C | -0.242117 | -1.693563 | -0.000000 |
| C | -0.242117 | 1.693563 | -0.000000 |
| C | -1.344388 | -1.056745 | -0.000000 |
| C | -1.344388 | 1.056745 | -0.000000 |
| H | 2.208818 | -1.490452 | 0.000000 |
| H | 2.208818 | 1.490452 | 0.000000 |
| H | 0.184083 | 2.657836 | 0.000000 |
| H | 0.184083 | -2.657836 | 0.000000 |
| H | -2.393838 | 1.168625 | -0.000000 |
| H | -2.393838 | -1.168625 | -0.000000 |

| | | | |
|---|---|---|---|
| C | 1.568217 | 0.638969 | 0.000000 |
| C | 1.568217 | -0.638969 | 0.000000 |
| C | -0.231124 | -1.678648 | -0.000000 |
| C | -0.231124 | 1.678648 | -0.000000 |
| C | -1.337021 | -1.039733 | -0.000000 |
| C | -1.337021 | 1.039733 | -0.000000 |
| H | 2.207943 | -1.480081 | 0.000000 |
| H | 2.207943 | 1.480081 | 0.000000 |
| H | 0.175624 | 2.651849 | 0.000000 |
| H | 0.175624 | -2.651849 | 0.000000 |
| H | -2.384443 | 1.172985 | -0.000000 |
| H | -2.384443 | -1.172985 | -0.000000 |

| | | | |
|---|---|---|---|
| C | 1.549995 | 0.641087 | 0.000000 |
| C | 1.549995 | -0.641087 | 0.000000 |
| C | -0.220179 | -1.663870 | -0.000000 |
| C | -0.220179 | 1.663870 | -0.000000 |
| C | -1.329749 | -1.022832 | -0.000000 |
| C | -1.329749 | 1.022832 | -0.000000 |
| H | 2.206853 | -1.469471 | 0.000000 |
| H | 2.206853 | 1.469471 | 0.000000 |
| H | 0.167068 | 2.645556 | 0.000000 |
| H | 0.167068 | -2.645556 | 0.000000 |
| H | -2.374732 | 1.177277 | -0.000000 |
| H | -2.374732 | -1.177277 | -0.000000 |

| | | | |
|---|---|---|---|
| C | 1.531942 | 0.643230 | 0.000000 |
| C | 1.531942 | -0.643230 | 0.000000 |
| C | -0.209297 | -1.649250 | -0.000000 |
| C | -0.209297 | 1.649250 | -0.000000 |
| C | -1.322583 | -1.006065 | -0.000000 |
| C | -1.322583 | 1.006065 | -0.000000 |
| H | 2.205547 | -1.458663 | 0.000000 |
| H | 2.205547 | 1.458663 | 0.000000 |
| H | 0.158450 | 2.638979 | 0.000000 |
| H | 0.158450 | -2.638979 | 0.000000 |
| H | -2.364743 | 1.181481 | -0.000000 |
| H | -2.364743 | -1.181481 | -0.000000 |

| | | | |
|---|---|---|---|
| C | 1.514062 | 0.645399 | 0.000000 |
| C | 1.514062 | -0.645399 | 0.000000 |
| C | -0.198480 | -1.634792 | -0.000000 |
| C | -0.198480 | 1.634792 | -0.000000 |
| C | -1.315526 | -0.989436 | -0.000000 |
| C | -1.315526 | 0.989436 | -0.000000 |
| H | 2.204020 | -1.447680 | 0.000000 |
| H | 2.204020 | 1.447680 | 0.000000 |
| H | 0.149792 | 2.632124 | 0.000000 |
| H | 0.149792 | -2.632124 | 0.000000 |
| H | -2.354492 | 1.185580 | -0.000000 |
| H | -2.354492 | -1.185580 | -0.000000 |

| | | | |
|---|---|---|---|
| C | 1.496356 | 0.647592 | 0.000000 |
| C | 1.496356 | -0.647592 | 0.000000 |
| C | -0.187726 | -1.620495 | -0.000000 |
| C | -0.187726 | 1.620495 | -0.000000 |
| C | -1.308578 | -0.972944 | -0.000000 |
| C | -1.308578 | 0.972944 | -0.000000 |
| H | 2.202269 | -1.436542 | 0.000000 |
| H | 2.202269 | 1.436542 | 0.000000 |
| H | 0.141115 | 2.624999 | 0.000000 |
| H | 0.141115 | -2.624999 | 0.000000 |
| H | -2.343995 | 1.189562 | -0.000000 |
| H | -2.343995 | -1.189562 | -0.000000 |

| | | | |
|---|---|---|---|
| C | 1.478821 | 0.649812 | 0.000000 |
| C | 1.478821 | -0.649812 | 0.000000 |
| C | -0.177037 | -1.606359 | -0.000000 |
| C | -0.177037 | 1.606359 | -0.000000 |
| C | -1.301738 | -0.956587 | -0.000000 |
| C | -1.301738 | 0.956587 | -0.000000 |
| H | 2.200289 | -1.425271 | 0.000000 |
| H | 2.200289 | 1.425271 | 0.000000 |
| H | 0.132436 | 2.617610 | 0.000000 |
| H | 0.132436 | -2.617610 | 0.000000 |
| H | -2.333269 | 1.193413 | -0.000000 |
| H | -2.333269 | -1.193413 | -0.000000 |

| | | | |
|---|---|---|---|
| C | 1.461454 | 0.652060 | 0.000000 |
| C | 1.461454 | -0.652060 | 0.000000 |
| C | -0.166407 | -1.592381 | -0.000000 |
| C | -0.166407 | 1.592381 | -0.000000 |
| C | -1.295006 | -0.940363 | -0.000000 |
| C | -1.295006 | 0.940363 | -0.000000 |
| H | 2.198079 | -1.413885 | 0.000000 |
| H | 2.198079 | 1.413885 | 0.000000 |
| H | 0.123776 | 2.609965 | 0.000000 |
| H | 0.123776 | -2.609965 | 0.000000 |
| H | -2.322328 | 1.197120 | -0.000000 |
| H | -2.322328 | -1.197120 | -0.000000 |

| | | | |
|---|---|---|---|
| C | 1.444251 | 0.654336 | 0.000000 |
| C | 1.444251 | -0.654336 | 0.000000 |
| C | -0.155835 | -1.578558 | -0.000000 |
| C | -0.155835 | 1.578558 | -0.000000 |
| C | -1.288382 | -0.924266 | -0.000000 |
| C | -1.288382 | 0.924266 | -0.000000 |
| H | 2.195634 | -1.402406 | 0.000000 |
| H | 2.195634 | 1.402406 | 0.000000 |
| H | 0.115150 | 2.602073 | 0.000000 |
| H | 0.115150 | -2.602073 | 0.000000 |
| H | -2.311190 | 1.200672 | -0.000000 |
| H | -2.311190 | -1.200672 | -0.000000 |

| | | | |
|---|---|---|---|
| C | 1.427207 | 0.656642 | 0.000000 |
| C | 1.427207 | -0.656642 | 0.000000 |
| C | -0.145316 | -1.564887 | -0.000000 |
| C | -0.145316 | 1.564887 | -0.000000 |
| C | -1.281864 | -0.908293 | -0.000000 |
| C | -1.281864 | 0.908293 | -0.000000 |
| H | 2.192954 | -1.390850 | 0.000000 |
| H | 2.192954 | 1.390850 | 0.000000 |
| H | 0.106577 | 2.593940 | 0.000000 |
| H | 0.106577 | -2.593940 | 0.000000 |
| H | -2.299869 | 1.204058 | -0.000000 |
| H | -2.299869 | -1.204058 | -0.000000 |

| | | | |
|---|---|---|---|
| C | 1.410316 | 0.658980 | 0.000000 |
| C | 1.410316 | -0.658980 | 0.000000 |
| C | -0.134846 | -1.551362 | -0.000000 |
| C | -0.134846 | 1.551362 | -0.000000 |
| C | -1.275449 | -0.892436 | -0.000000 |
| C | -1.275449 | 0.892436 | -0.000000 |
| H | 2.190039 | -1.379237 | 0.000000 |
| H | 2.190039 | 1.379237 | 0.000000 |
| H | 0.098073 | 2.585576 | 0.000000 |
| H | 0.098073 | -2.585576 | 0.000000 |
| H | -2.288380 | 1.207269 | -0.000000 |
| H | -2.288380 | -1.207269 | -0.000000 |

| | | | |
|---|---|---|---|
| C | 1.393572 | 0.661351 | 0.000000 |
| C | 1.393572 | -0.661351 | 0.000000 |
| C | -0.124419 | -1.537981 | -0.000000 |
| C | -0.124419 | 1.537981 | -0.000000 |
| C | -1.269136 | -0.876689 | -0.000000 |
| C | -1.269136 | 0.876689 | -0.000000 |
| H | 2.186887 | -1.367585 | 0.000000 |
| H | 2.186887 | 1.367585 | 0.000000 |
| H | 0.089653 | 2.576988 | 0.000000 |
| H | 0.089653 | -2.576988 | 0.000000 |
| H | -2.276738 | 1.210295 | -0.000000 |
| H | -2.276738 | -1.210295 | -0.000000 |

| | | | |
|---|---|---|---|
| C | 1.376966 | 0.663758 | 0.000000 |
| C | 1.376966 | -0.663758 | 0.000000 |
| C | -0.114031 | -1.524735 | -0.000000 |
| C | -0.114031 | 1.524735 | -0.000000 |
| C | -1.262924 | -0.861044 | -0.000000 |
| C | -1.262924 | 0.861044 | -0.000000 |
| H | 2.183498 | -1.355909 | 0.000000 |
| H | 2.183498 | 1.355909 | 0.000000 |
| H | 0.081330 | 2.568186 | 0.000000 |
| H | 0.081330 | -2.568186 | 0.000000 |
| H | -2.264959 | 1.213127 | -0.000000 |
| H | -2.264959 | -1.213127 | -0.000000 |

| | | | |
|---|---|---|---|
| C | 1.360491 | 0.666203 | 0.000000 |
| C | 1.360491 | -0.666203 | 0.000000 |
| C | -0.103676 | -1.511621 | -0.000000 |
| C | -0.103676 | 1.511621 | -0.000000 |
| C | -1.256810 | -0.845494 | -0.000000 |
| C | -1.256810 | 0.845494 | -0.000000 |
| H | 2.179873 | -1.344227 | 0.000000 |
| H | 2.179873 | 1.344227 | 0.000000 |
| H | 0.073119 | 2.559178 | 0.000000 |
| H | 0.073119 | -2.559178 | 0.000000 |
| H | -2.253057 | 1.215759 | -0.000000 |
| H | -2.253057 | -1.215759 | -0.000000 |

| | | | |
|---|---|---|---|
| C | 1.344137 | 0.668688 | 0.000000 |
| C | 1.344137 | -0.668688 | 0.000000 |
| C | -0.093347 | -1.498631 | -0.000000 |
| C | -0.093347 | 1.498631 | -0.000000 |
| C | -1.250791 | -0.830030 | -0.000000 |
| C | -1.250791 | 0.830030 | -0.000000 |
| H | 2.176013 | -1.332553 | 0.000000 |
| H | 2.176013 | 1.332553 | 0.000000 |
| H | 0.065032 | 2.549972 | 0.000000 |
| H | 0.065032 | -2.549972 | 0.000000 |
| H | -2.241044 | 1.218183 | -0.000000 |
| H | -2.241044 | -1.218183 | -0.000000 |

| | | | |
|---|---|---|---|
| C | 1.327896 | 0.671216 | 0.000000 |
| C | 1.327896 | -0.671216 | 0.000000 |
| C | -0.083036 | -1.485759 | -0.000000 |
| C | -0.083036 | 1.485759 | -0.000000 |
| C | -1.244865 | -0.814641 | -0.000000 |
| C | -1.244865 | 0.814641 | -0.000000 |
| H | 2.171919 | -1.320902 | 0.000000 |
| H | 2.171919 | 1.320902 | 0.000000 |
| H | 0.057081 | 2.540577 | 0.000000 |
| H | 0.057081 | -2.540577 | 0.000000 |
| H | -2.228934 | 1.220395 | -0.000000 |
| H | -2.228934 | -1.220395 | -0.000000 |

| | | | |
|---|---|---|---|
| C | 1.311757 | 0.673789 | 0.000000 |
| C | 1.311757 | -0.673789 | 0.000000 |
| C | -0.072737 | -1.472997 | -0.000000 |
| C | -0.072737 | 1.472997 | -0.000000 |
| C | -1.239030 | -0.799318 | -0.000000 |
| C | -1.239030 | 0.799318 | -0.000000 |
| H | 2.167594 | -1.309287 | 0.000000 |
| H | 2.167594 | 1.309287 | 0.000000 |
| H | 0.049276 | 2.531001 | 0.000000 |
| H | 0.049276 | -2.531001 | 0.000000 |
| H | -2.216740 | 1.222388 | -0.000000 |
| H | -2.216740 | -1.222388 | -0.000000 |

| | | | |
|---|---|---|---|
| C | 1.295710 | 0.676411 | 0.000000 |
| C | 1.295710 | -0.676411 | 0.000000 |
| C | -0.062443 | -1.460337 | -0.000000 |
| C | -0.062443 | 1.460337 | -0.000000 |
| C | -1.233283 | -0.784051 | -0.000000 |
| C | -1.233283 | 0.784051 | -0.000000 |
| H | 2.163039 | -1.297721 | 0.000000 |
| H | 2.163039 | 1.297721 | 0.000000 |
| H | 0.041625 | 2.521253 | 0.000000 |
| H | 0.041625 | -2.521253 | 0.000000 |
| H | -2.204474 | 1.224159 | -0.000000 |
| H | -2.204474 | -1.224159 | -0.000000 |

| | | | |
|---|---|---|---|
| C | 1.279743 | 0.679084 | 0.000000 |
| C | 1.279743 | -0.679084 | 0.000000 |
| C | -0.052144 | -1.447772 | -0.000000 |
| C | -0.052144 | 1.447772 | -0.000000 |
| C | -1.227621 | -0.768827 | -0.000000 |
| C | -1.227621 | 0.768827 | -0.000000 |
| H | 2.158258 | -1.286215 | 0.000000 |
| H | 2.158258 | 1.286215 | 0.000000 |
| H | 0.034139 | 2.511340 | 0.000000 |
| H | 0.034139 | -2.511340 | 0.000000 |
| H | -2.192147 | 1.225704 | -0.000000 |
| H | -2.192147 | -1.225704 | -0.000000 |

| | | | |
|---|---|---|---|
| C | 1.263846 | 0.681811 | 0.000000 |
| C | 1.263846 | -0.681811 | 0.000000 |
| C | -0.041832 | -1.435294 | -0.000000 |
| C | -0.041832 | 1.435294 | -0.000000 |
| C | -1.222041 | -0.753636 | -0.000000 |
| C | -1.222041 | 0.753636 | -0.000000 |
| H | 2.153254 | -1.274781 | 0.000000 |
| H | 2.153254 | 1.274781 | 0.000000 |
| H | 0.026825 | 2.501272 | 0.000000 |
| H | 0.026825 | -2.501272 | 0.000000 |
| H | -2.179770 | 1.227021 | -0.000000 |
| H | -2.179770 | -1.227021 | -0.000000 |

| | | | |
|---|---|---|---|
| C | 1.248007 | 0.684597 | 0.000000 |
| C | 1.248007 | -0.684597 | 0.000000 |
| C | -0.031499 | -1.422893 | -0.000000 |
| C | -0.031499 | 1.422893 | -0.000000 |
| C | -1.216539 | -0.738466 | -0.000000 |
| C | -1.216539 | 0.738466 | -0.000000 |
| H | 2.148031 | -1.263428 | 0.000000 |
| H | 2.148031 | 1.263428 | 0.000000 |
| H | 0.019689 | 2.491056 | 0.000000 |
| H | 0.019689 | -2.491056 | 0.000000 |
| H | -2.167353 | 1.228108 | -0.000000 |
| H | -2.167353 | -1.228108 | -0.000000 |

| | | | |
|---|---|---|---|
| C | 1.232212 | 0.687444 | 0.000000 |
| C | 1.232212 | -0.687444 | 0.000000 |
| C | -0.021135 | -1.410562 | -0.000000 |
| C | -0.021135 | 1.410562 | -0.000000 |
| C | -1.211113 | -0.723303 | -0.000000 |
| C | -1.211113 | 0.723303 | -0.000000 |
| H | 2.142592 | -1.252166 | 0.000000 |
| H | 2.142592 | 1.252166 | 0.000000 |
| H | 0.012737 | 2.480700 | 0.000000 |
| H | 0.012737 | -2.480700 | 0.000000 |
| H | -2.154908 | 1.228964 | -0.000000 |
| H | -2.154908 | -1.228964 | -0.000000 |

| | | | |
|---|---|---|---|
| C | 1.216451 | 0.690356 | 0.000000 |
| C | 1.216451 | -0.690356 | 0.000000 |
| C | -0.010731 | -1.398291 | -0.000000 |
| C | -0.010731 | 1.398291 | -0.000000 |
| C | -1.205761 | -0.708137 | -0.000000 |
| C | -1.205761 | 0.708137 | -0.000000 |
| H | 2.136942 | -1.241005 | 0.000000 |
| H | 2.136942 | 1.241005 | 0.000000 |
| H | 0.005975 | 2.470214 | 0.000000 |
| H | 0.005975 | -2.470214 | 0.000000 |
| H | -2.142444 | 1.229588 | -0.000000 |
| H | -2.142444 | -1.229588 | -0.000000 |

| | | | |
|---|---|---|---|
| C | 1.200711 | 0.693338 | 0.000000 |
| C | 1.200711 | -0.693338 | 0.000000 |
| C | -0.000276 | -1.386073 | -0.000000 |
| C | -0.000276 | 1.386073 | -0.000000 |
| C | -1.200479 | -0.692953 | -0.000000 |
| C | -1.200479 | 0.692953 | -0.000000 |
| H | 2.131089 | -1.229954 | 0.000000 |
| H | 2.131089 | 1.229954 | 0.000000 |
| H | -0.000591 | 2.459608 | -0.000000 |
| H | -0.000591 | -2.459608 | -0.000000 |
| H | -2.129973 | 1.229981 | -0.000000 |
| H | -2.129973 | -1.229981 | -0.000000 |
